# Supplementary material for: Version Age of Information Minimization over Fading Broadcast Channels
Source: arXiv:2311.09975 source file (2024-02-12)
Supplement: Supplementary file 1 [file Appendix.tex]

We now prove the second part of the theorem. 
Suppose it is optimal to transmit stream $i$ for some $h_i$, $\mathbf{h}_{-i}$, $\boldsymbol{\Delta}$ and $\mathbf{u}_{-i}$. This means that 
\begin{align}
Q(h_i, 1,\cdot) - Q(h_i, 0,\cdot) <0,  
\end{align}
where we replace $\mathbf{h_{-i}}$, $\boldsymbol{\Delta}$ and $\mathbf{u}_{-i}$ with a $(\cdot)$ for brevity. Then, for proving the second part of the theorem, it is sufficient to show that: $Q(h_i+\epsilon, 1,\cdot) - Q(h_i+\epsilon, 0,\cdot) <0$ for any $\epsilon>0$, which we accomplish in the below. Consider
\begin{align}
&Q(h_i+\epsilon, 1,\cdot) - Q(h_i+\epsilon, 0,\cdot)  \\
& = \mathbb{E}_{A}\left[C(h_i+\epsilon , 1,\cdot)\right] + \gamma \mathbb{E}_{A,H}\left[v(0, \boldsymbol{\Delta'_{-i}}, \mathbf{h}'|h_i+\epsilon ,1,\cdot)\right] \nonumber\\
&\;\;\;\; - \mathbb{E}_A\left[C(h_i+\epsilon , 0,\cdot)\right] - \gamma\mathbb{E}_{A,H}\left[v(\Delta_i', \boldsymbol{\Delta'_{-i}}, \mathbf{h}'|h_i+\epsilon ,0,\cdot)\right]\\
& = \mathbb{E}_A\left[0 +\beta P_i+ \sum_{j \neq i}w_j\Delta'_j+\beta u_jP_j|h_i+\epsilon ,1,\cdot\right]+
\gamma\mathbb{E}_{A,H}\left[v(0, \boldsymbol{\Delta}'_{-i}, \mathbf{h}'|h_i+\epsilon ,1,\cdot)\right] \nonumber\\
&\;\;\;\;  -  \sum_{j}\mathbb{E}_A\left[w_j{\Delta}'_j+\beta u_jP_j|h_i+\epsilon ,0,\cdot\right]-\gamma\mathbb{E}_{A,H}\left[v(\Delta_i', \boldsymbol{\Delta'_{-i}}, \mathbf{h}'|h_i+\epsilon ,0, \cdot)\right]\label{eq:last_high_h}\\
&\stackrel{(a)}{\leq} \mathbb{E}_A\left[ 0 +\beta P_i+ \sum_{j \neq i}w_j\Delta'_j+\beta u_jP_j|h_i,1,\cdot\right]+
\gamma\mathbb{E}_{A,H}\left[v(0, \boldsymbol{\Delta'_{-i}}, \mathbf{h}'|h_i,1,\cdot)\right] \nonumber\\
&\;\;\;\;   -  \sum_{j}\mathbb{E}_A\left[w_j\Delta'_j+\beta u_jP_j|h_i,0,\cdot\right]-\gamma\mathbb{E}_{A,H}\left[v(\Delta_i', \boldsymbol{\Delta'_{-i}}, \mathbf{h}'|h_i,0, \cdot)\right]\label{eq:first_low_h}\\
& = \mathbb{E}_{A}\left[C(\Delta_i, 1,\cdot)\right] + \gamma \mathbb{E}_{A,H}\left[v(0, \boldsymbol{\Delta'_{-i}}, \mathbf{h}'|h_i,1,\cdot)\right] \nonumber\\
&\;\;\;\;  - \mathbb{E}_A\left[C(\Delta_i, 0,\cdot)\right] - \gamma\mathbb{E}_{A,H}\left[v(\Delta_i', \boldsymbol{\Delta'_{-i}}, \mathbf{h}'|h_i,0,\cdot)\right]\\
&=Q(h_i, 1,\cdot) - Q(h_i, 0,\cdot), 
\end{align}
where (a) is because (i) $\mathbb{E}_{A,H}\left[v(0, \boldsymbol{\Delta}'_{-i}, \mathbf{h}'|h_i+\epsilon ,1,\cdot)\right]=\mathbb{E}_{A,H}\left[v(0, \boldsymbol{\Delta}'_{-i}, \mathbf{h}'|h_i,1,\cdot)\right]$ as channel power gains transition independently across slots, and when a packet from stream $i$ is transmitted, the VAoI component of stream $i$ in the next transition will be zero and other VAoIs evolve identically irrespective of whether the channel power gain is $h_i+\epsilon$ or $h_i$, (ii) the last two terms of \eqref{eq:last_high_h} and the last two terms of \eqref{eq:first_low_h} are identical as if we do not transmit a packet in stream $i$, when all other state and action components remain the same, both VAoI and power consumption remain the same irrespective of the channel of user $i$ being $h_i+\epsilon$ or $h_i$, and the channels evolve independently, (iii) $\mathbb{E}_A\left[0 +\beta P_i+ \sum_{j \neq i}w_j\Delta'_j+\beta u_jP_j|h_i+\epsilon ,1,\cdot\right]\leq \mathbb{E}_A\left[0 +\beta P_i+ \sum_{j \neq i}w_j\Delta'_j+\beta u_jP_j|h_i ,1,\cdot\right]$, which we prove in the lemma below.

\begin{lemma}
$\mathbb{E}_A\left[0 +\beta P_i+ \sum_{j \neq i}w_j\Delta'_j+\beta u_jP_j|h_i+\epsilon ,1,\cdot\right]\leq \mathbb{E}_A\left[0 +\beta P_i+ \sum_{j \neq i}w_j\Delta'_j+\beta u_jP_j|h_i ,1,\cdot\right]$ holds. 
\end{lemma}
\begin{proof}

Note that, 
       \begin{align}
           &\mathbb{E}_A\left[0 +\beta P_i+ \sum_{j \neq i}w_j\Delta'_j+\beta u_jP_j|h_i + \epsilon,1,\cdot\right] \nonumber \\
           &\leq \mathbb{E}_A\left[0 +\beta P_i+ \sum_{j \neq i}w_j\Delta'_j+\beta u_jP_j|h_i ,1,\cdot\right] \\
           \implies& \mathbb{E}_A\left[\sum_{j \neq i} w_j \Delta_j' | \boldsymbol{u} \right] + \left[\beta P_i + \sum_{j \neq i} \beta u_jP_j| h_i + \epsilon, 1, \cdot \right]  \nonumber\\
           & \leq \mathbb{E}_A\left[\sum_{j \neq i} w_j \Delta_j' | \boldsymbol{u} \right] + \left[\beta P_i + \sum_{j \neq i} \beta u_jP_j| h_i, 1, \cdot \right] \\
           \implies& \left[\beta P_i + \sum_{j \neq i} \beta u_jP_j| h_i + \epsilon, 1, \cdot \right] \leq \left[\beta P_i + \sum_{j \neq i} \beta u_jP_j| h_i, 1, \cdot \right] 
           % \implies& \left[\beta P_i + \sum_{j \geq i} \beta u_jP_j| h_i + \epsilon, 1, \cdot \right]  \leq \left[\beta P_i + \sum_{j \geq i} \beta u_jP_j| h_i, 1, \cdot \right] 
       \end{align}

        Equation 31 implies 32 since the weighted sum of VAoI's of the n streams depends only on the action and not the realisation of h.

	Let 
        \begin{align*}
        & h_1\geq h_2\geq \ldots h_{i-1} \geq h_{i}+\epsilon\geq h_{i+1}\geq \ldots\geq h_N \\
        & h_1\geq h_2\geq \ldots h_{i-1} \geq h_{i} \geq h_{i+1}\geq \ldots\geq h_N
        \end{align*}

    We know that:

\begin{align*}
P_{O_1}u_{O_1}&= \frac{f^{-1}\left(R^0_{O_1}u_{O_1}\right)}{h_{O_1}}\label{eq:TransmitPower1}\\
P_{O_2}u_{O_2}&= \frac{f^{-1}\left(R^0_{O_2}u_{O_2}\right)}{h_{O_2}}+\nonumber\\
&\;\;f^{-1}\left(R^0_{O_2}u_{O_2}\right)\frac{f^{-1}\left(R^0_{O_1}u_{O_1}\right)}{h_{O_1}},
\\
&\ldots\nonumber \\
P_{O_i}u_{O_i} &= \frac{f^{-1}\left( R^{0}_{O_i} u_{O_i} \right)}{h_{O_i}} + f^{-1}\left( R^{0}_{O_i} u_{O_i} \right) \sum_{k=1}^{i-1}P_{O_k}u_{O_k}
\end{align*}

Hence, $[P_i|h_i + \epsilon, 1, \cdot] < [P_i|h_i, 1, \cdot]$, since $h_i$ is in the denominator. Also, $[P_j|h_i + \epsilon, 1, \cdot] < [P_j|h_i, 1, \cdot] \; \forall \; j>i$, since each $P_j$ contains the sum of the previous transmit powers from $P_1, \ldots, P_{j-1}$. We also have $[P_j|h_i + \epsilon, 1, \cdot] = [P_j|h_i, 1, \cdot] \; \forall \; j<i$, since the values of $h_j$ are same $\forall j<i$

So, in this case, equation 33 holds.

Now, consider the case where epsilon is large enough such that,
        \begin{align*}
        & h_1\geq h_2\geq \ldots h_{i}+\epsilon\geq h_k \geq\ldots h_{i-1} \geq h_{i+1}\geq \ldots\geq h_N  \\
        & h_1\geq h_2\geq \ldots h_{i-1} \geq h_{i} \geq h_{i+1}\geq \ldots\geq h_N 
        \end{align*}

        for some $k<i$

        Suppose $\boldsymbol{h^*}$ be the new channel gain vector, such that,
        % \begin{align*}
        %     &h_j^* = h_j \;\;\; \forall j \leq k-1 \\
        %     &h_k^* = h_i \\
        %     &h_j^* = h_{j-1} \;\;\; \forall  k+1 \leq j \leq i \\
        %     &h_j^* = h_j  \;\;\; \forall j > i \\
        % \end{align*}

        $$
        h_j^* = 
        \begin{cases}
            h_j &  j \leq k-1 \text{ and }  j > i\\
            h_i + \epsilon & j=k \\
            h_{j-1} &   k+1 \leq j \leq i \\
        \end{cases}
        $$

                In this case, following are the channel numbers and their corresponding channel gains:

        \begin{center}
        \small\addtolength{\tabcolsep}{-5pt}
        \begin{tabular}{ |c|c|c|c|c|c|c|c|c|c|c|c| } 
         \hline
         1 & 2 & $\ldots$ & $k-1$ & $k$ & $k+1$ & $\ldots$ & $i-1$ & $i$ & $i+1$& $\ldots$ & $N$ \\
         \hline
         $h_1^*$ & $h_2^*$ & $\ldots$ & $h_{k-1}^*$ & $h_k^*$ & $h_{k+1}^*$ & $\ldots$ & $h_{i-1}^*$ & $h_i^*$ & $h_{i+1}^*$& $\ldots$ & $h_N^*$ \\
         \hline
         $h_1$ & $h_2$ & $\ldots$ & $h_{k-1}$ & $h_i + \epsilon$ & $h_k$ & $\ldots$ & $h_{i-2}$ & $h_{i-1} $ & $h_{i+1}$ & $\ldots$ & $h_N$ \\ 
         \hline
        \end{tabular}
        \end{center}

        Now,  $[P_j|h_i + \epsilon, 1, \cdot] = [P_j|h_i, 1, \cdot] \;\;\; \forall j<k$ since  $h_j^* = h_j \;\;\; \forall j<k$ 
        .

        Also, $h_i+\epsilon > h_k \implies h_k^* > h_k$
        So, $[P_i|h_i + \epsilon, 1, \cdot] < [P_i|h_i, 1, \cdot]$

        Similarly, 
        \begin{align*}
            &h_{j-1} > h_j \;\;\; \forall \;\; k+1\leq j \leq i \\
            \implies &h_j^* > h_j \;\;\; \forall \;\; k+1\leq j \leq i \\ 
        \end{align*}

        Hence, $[P_j|h_i + \epsilon, 1, \cdot] < [P_j|h_i, 1, \cdot] \;\;\; \forall k+1\leq j \leq i$ \\

        Now, for $j>i$, we have $h_j^* = h_j$. But the transmit power of the $j$th channel contains the sum of the transmit powers of the previous channels $1, \ldots, j-1$. Hence, we have,
$[P_j|h_i + \epsilon, 1, \cdot] < [P_j|h_i, 1, \cdot] \;\;\; \forall \;\; j > i$ \\

        Therefore, in this case too, equation 33 holds true.

\end{proof}
